# Supplementary material for: TableLlama: Towards Open Large Generalist Models for Tables
Source: arXiv:2311.09206 source file (2024-04-04)
Supplement: Supplementary file 1 [file appendix_v1.tex]

\section{Appendix.}

\begin{algorithm}[!htbp]
\caption{Pseudo code of Dynamic Subtable Segmentation}
\label{algo1}
\KwIn{Segmented subtable set: $sub\_tab\_set = \emptyset$. $input$ contains prompt, table metadata, $table$ and instruction. Initialize the maximum input length: $L_{max}$, reserved prompt length: $L_{pro}$, reserved instruction length: $L_{ins}$, reserved table metadata length: $L_{meta}$ for each task and the offset. Denote input length as $L_{inp}$ and serialized table length as $L_{tab}$. Note all lengths here refer to the length after tokenization, rather than the original string length.}
\KwOut{the final subtable set $S$.}
$L_{inp} = L_{pro} + L_{meta} + L_{tab} + L_{ins}$ \\
\If{$L_{inp} > L_{max}$}
{
$seg\_tab\_num = \lceil L_{tab} / (L_{max} - L_{pro} - L_{ins} - L_{meta} - $ offset$) \rceil$ TO EXPLAIN THIS \\
\For{$i\in1,2, ..., seg\_tab\_num$}
{
\If{$i=1$}
{
$start\_idx = 0$ \\
$end\_idx = L_{max} - L_{ins} - L_{pro} - L_{meta}$ \\
}
\Else
{
$start\_idx = end\_idx - $ offset \\
$end\_idx = start\_idx + L_{max} - L_{ins} - L_{pro} - L_{meta}$\\
}
$sub\_table\_set = sub\_table\_set \cup table[start\_idx: end\_idx]$ \\
}   
}
\Else
{
$sub\_table\_set = input$ \\
}
return $sub\_table\_set$
\end{algorithm}

\begin{algorithm}[H]
\caption{Pseudo code of Tree Rank (for each sublayer)}
\label{algo3}
\KwIn{Subsets needed to be ranked: $\{\displaystyle \sA_1, \displaystyle \sA_2,... \displaystyle \sA_n\}$. Optional: single half $H^f$ and $H^b$ from last layer.}
\KwOut{The merged front halves $\{\displaystyle \sA^f_1, \displaystyle \sA^f_2,... \displaystyle \sA^f_{n/2}\}$ and the merged bottom halves $\{\displaystyle \sA^b_1, \displaystyle \sA^b_2,... \displaystyle \sA^b_{n/2}\}$. Optional: the last subset half $H^f_n$ and $H^b_n$.}
{
% Reinitialize the number of the subset $n$. \\
Let the model rank each subset $\displaystyle \sA_i$. \\
Divide elements of each ranked subset into two halves based on the order: the front half $H^f_i$ and the bottom half $H^b_i$, $i\in \{1,2,...,n\}$. \\
\If{$n\%2 == 0$}
{
Merge all the front halves $H^f_i$ in pairs and get the new subsets: $\displaystyle \sA^f_k$, $\displaystyle \sA^f_k = H^f_i\cup H^f_{i+1}$. \\ 
Merge all the bottom halves $H^b_i$ in pairs and get the new subsets: $\displaystyle \sA^b_k$, $\displaystyle \sA^b_k = H^b_i\cup H^b_{i+1}$. \\ 
Get all the merged front halves $\{\displaystyle \sA^f_1, \displaystyle \sA^f_2,... \displaystyle \sA^f_{n/2}\}$
and all the merged bottom halves $\{\displaystyle \sA^b_1, \displaystyle \sA^b_2,... \displaystyle \sA^b_{n/2}\}$.
}
\Else{
Merge all the front halves $H^f_i$ in pairs and get the new subsets: $\displaystyle \sA^f_k$ except the last half $H^f_n$. \\ 
Merge all the bottom halves $H^b_i$ in pairs and get the new subsets: $\displaystyle \sA^b_k$ except the last half $H^b_n$.\\ 
Get all the merged front halves $\{\displaystyle \sA^f_1, \displaystyle \sA^f_2,... \displaystyle \sA^f_{(n-1)/2}\}$ and all the merged bottom halves $\{\displaystyle \sA^b_1, \displaystyle \sA^b_2,... \displaystyle \sA^b_{(n-1)/2}\}$. \\
\If{
$H^f$ exists and $H^b$ exists
}
{
Merge $H^f$ and $H^f_n$ to be $\displaystyle \sA^f_{n/2}$. Merge $H^b$ and $H^b_n$ to be $\displaystyle \sA^b_{n/2}$. 
}
\Else{
Convey the last subset half $H^f_n$ and $H^b_n$ to the next layer. 
}
}
Make sure all the merged front halves $\{\displaystyle \sA^f_1, \displaystyle \sA^f_2,... \displaystyle \sA^f_{n/2}\}$
are in front of all the merged bottom halves $\{\displaystyle \sA^b_1, \displaystyle \sA^b_2,... \displaystyle \sA^b_{n/2}\}$.
}

\end{algorithm}

To be specific, for Alpaca and LLaMA2, the prompt is ``Below is an instruction that describes a task, paired with an input that provides further context. Write a response that appropriately completes the request". For Vicuna, the prompt is ``A chat between a curious user and an artificial intelligence assistant. The assistant gives helpful, detailed, and polite answers to the user's questions." \\
 The ``Input" part is mainly for table-related information. We start with a special token ``[TLE]", followed by the table metadata (Wikipedia page title, Wikipedia section title and table caption) and serialized table headers and contents. We use a special token ``[TAB]" to start the table headers and use a special token ``[SEP]" to separate each row of the table contents. For schema augmentation and row population, our goal is to populate the model to generate the suggested following table headers or following table subject columns, so we don't input table contents for them. For schema augmentation, we only input table metadata and one seed header. For row population, we input table metadata, table headers and one entity of the subject column. For FeTaQA which the model tries to answer the questions in a free form based on the highlighted cells, we use special tokens ``[HIGHTED\_BEGIN]" and ``[HIGHTED\_END]" to explicitly highlight the related table cells. \\
 The ``Instruction" part is the most different part for different tasks. For column type annotation, we pick an entity from the target column and give the column name. Then we provide the type candidates followed by a question to ask the column type of this entity. For relation extraction, we pick an entity pair from the target column pair and give the column names of these two entities. Then we provide the relation candidates followed by a question to ask the relation of this entity pair. For entity linking, we give the model the task description and provide the entity candidates. Each entity candidate format is the ``entity name [Description] entity description". Then we provide a question to ask the best match of the entity mention from the entity candidates. For schema augmentation and row population, we provide the task description and ask the model to rank the given candidates. For Spreadsheet QA and free-form QA, the instruction is the question. For fact verification, the instruction is the task description and given a statement, let the model distinguish whether it's entailed or refuted.

Important to give more details (descriptions) for each task. especially for the instruction part. What the types look like, referent entity look like, how we organize the instruction, also refer to figure 1 and echo it.
